# Supplementary material for: A Database System for State Management in Stateful Network Service Function Chains [Vision]
Source: arXiv:2312.01066 source file (2023-12-02)
Supplement: Supplementary file 1 [file Appendix.tex]

% One page of the Appendix is allowed.
